# Supplementary material for: Achieving State Machine Replication without Honest Players
Source: arXiv:2012.10146 source file (2021-05-31)
Supplement: Supplementary file 1 [file Quotes.tex]

\section{Quotes}

\begin{itemize}
    \item \cite{GeneralFrameworkSecurityAnalysisBlockchain}: In the real world, users are not simply honest or otherwise, and a game theoretic analysis can give much more robust performance guarantees than reliance on the honesty of certain users.
    \item \cite{SoKConsensus}: incentivization in committee-based blockchain consensus protocols (with leader) has started to see some study, but is far from mature. This area will benefit from combining formal economic and game theoretic analysis with cryptography.
    \item \cite{SOKGameTheoryBlockchain}:  
    \begin{itemize}
        \item Game theory is natural in the decision making of all the consensus nodes in the blockchain networks. 
        \item The blockchain consensus protocol is expected to be incentive compatible.
    \end{itemize}
    \item \cite{SelfishMining}: Since Bitcoin mining is open to the public, oﬀering ﬁnancial rewards, we conjecture that altruistic miners are few.
    \item \cite{FruitChains}: Assuming honest participation, however, is a strong assumption, especially in a setting where honest players are expected to perform a lot of work.
    \item \cite{Fairledger}:  We have to take into account that every entity may behave rationally, and deviate from the protocol if doing so increases its benefit.
    \item \cite{Fairledger}: to prove that a protocol is correct in our model, we need to show that (1) the problem speciﬁcation is satisﬁed in case all the rational entities follow the protocol and there are at most f byzantine ones, and (2) following the protocol is an equilibrium for rational entities even in the presence of f byzantine ones.
    \item \cite{SoKToolsGameTheoryCryptocurrencies}:  having a system that is secure with some bounded number of Byzantine faults is not enough to have a decentralized system as decentralization cannot be assumed. Rather, incentives should be designed to ensure enough (honest) participation.
    \item \cite{Bitcoin}: As long as a majority of CPU power is controlled by nodes that are not cooperating to attack the network, they’ll generate the longest chain and outpace attackers.
    
\end{itemize}
